# Supplementary material for: Determining the phase diagram of atomically thin layered antiferromagnet CrCl$_3$
Source: arXiv:1911.04376 ancillary file (2019-11-11)
Supplement: Supplementary file 1 [file supplementary_information.pdf]

# Supplementary Materials for "*Determining the phase diagram of atomically thin layered antiferromagnet $CrCl_3$*"

Zhe Wang,[1,2] Marco Gibertini,[1,3] Dumitru Dumcenco,[1] Takashi Taniguchi,[4]
Kenji Watanabe,[4] Enrico Giannini,[1] and Alberto F. Morpurgo[1,2]

[1]*Department of Quantum Matter Physics, University of Geneva, 24 Quai Ernest Ansermet, CH-1211 Geneva, Switzerland*
[2]*Group of Applied Physics, University of Geneva, 24 Quai Ernest Ansermet, CH-1211 Geneva, Switzerland*
[3]*National Centre for Computational Design and Discovery of Novel Materials (MARVEL), École Polytechnique Fédérale de Lausanne, CH-1015 Lausanne, Switzerland*
[4]*National Institute for Materials Science, 1-1 Namiki, Tsukuba, 305-0044, Japan*
(Dated: May 16, 2019)

## Supplementary Note 1: Structural and stoichiometric characterization

We performed X-ray diffraction (XRD) and Energy-dispersive X-ray (EDX) spectroscopy measurements to confirm that the crystals grown by vapor phase transport actually have the expected structure and composition. For XRD characterization we used a powder diffractometer (Bruker D8 Advance with Cu-$K_{\alpha 1}$ monochromator for measurement in Bragg-Brentano reflection geometry). The pattern shows only one set of narrow [00l] reflections, compatible with the expected C12/m crystal structure, proving the high crystallinity of the sample (Supplementary Fig. 1). EDX analysis was performed in a JEOL JSM 7600F scanning electron microscope equipped with an Oxford SDD Max-80 X-ray detector. The SEM images show crystals with flat and clean surfaces and the EDX confirms a homogeneous atomic ratio Cr:Cl equal to 1:3. Even if a clearly detectable greenish powder is found on the hot side of the tube at the end of the growth (that we attribute to $Cr_2O_3$), EDX detected no trace of oxygen in the $CrCl_3$ crystals that we used for exfoliation.

## Supplementary Note 2: Bulk Magnetism

We performed measurements of magnetization as a function of magnetic field (up to $\mu_0 H$=7 T) at fixed temperature $T$, or as a function of $T$ in the presence of a small applied magnetic field ($\mu_0 H = 0.001$ T), using a MPMS3 SQUID magnetometer from Quantum Design (see Supplementary Fig. 2). The isothermal magnetization curves were collected after zero-field cooling (ZFC); the temperature dependent data were collected rising the temperature, both after ZFC and after field cooling (FC). Our observations generally agree with those reported in previous studies. Fig. 2(a) shows the magnetic moment as a function of in-plane and out-of-plane magnetic field at 1.8 K. At high field, the magnetic moment saturates at a value close to 3.0 $\mu_B$ per Cr atom, as expected (nearly complete saturation is reached already at an applied field of 0.2 T). The temperature dependence of the magnetic moment per Cr atom measured with a field of 0.001 T applied in-plane and out-of-plane is shown in Fig. 2(b) and (c), respectively. The curves are consistent with earlier measurements[1] and show that in bulk $CrCl_3$ the Néel temperature (associated with 3D interlayer antiferromangetic order) is $T_N \simeq 14.5$ K.

Note that the value of $T_N \simeq 17$ K measured in multilayers is overall larger than the bulk $T_N$ (see inset to Fig. 5 in the main text). This is consistent with the larger magnetic field scale observed for the spin-flip transition in multilayers ($\mu_0 H_2 \simeq 2$ T) with respect to the bulk spin-flip field $\mu_0 H_2^{\text{bulk}} \simeq 0.2$ T[1–3], which points to a larger interlayer exchange coupling in multilayers and thus a larger Néel temperature. The phenomenon likely originates from a different crystalline structure of atomically thin multilayers as compared to the bulk[4], suggesting that $T_N \simeq 14.5$ K is associated with the rhombohedral structure (that in bulk appears at low temperature) while $T_N \simeq 17$ K in the monoclinic phase typical of multilayers (that in bulk appears only at high temperature). This scenario would also explain the existence of a second anomaly in the heat capacity of bulk $CrCl_3$ close to $T \simeq 17$ K[1,5] if we assume that bulk crystals include regions (e.g. close to the surfaces) that remain in the high-temperature phase.

## Supplementary Note 3: Field-dependence of the magnetization configuration in bi- and trilayers

We show here how to derive the magnetic configuration of bi- and tri-layers as a function of magnetic field (applied parallel to the layers), reported in Fig. 3**a** and **b** of the main text.

When the field is applied in-plane, the combined effect of the external field and magnetic anisotropy is such that we can assume the magnetization in each layer to lie in-plane. Taking for definiteness the external field along the $x$-axis, this means that in the zero-temperature limit we can write the magnetization in the $i$-th layer as $\boldsymbol{M}_i = M_s(\cos\phi_i, \sin\phi_i, 0)$, so that the micromagnetic energy in Eq. (**??**) then reads:

$$U_N(\phi_1,\ldots,\phi_N;H) = J\sum_{i=1}^{N-1}\cos(\phi_{i+1}-\phi_i) - \mu_0 M_s H\sum_{i=1}^{N}\cos(\phi_i)\ , \tag{S1}$$

which corresponds to Eq. (1) in the main text. The most stable configuration for a given value of $H$ can be obtained by minimizing $U_N$, i.e. by looking for the lowest-energy solution to the following set of $N$ equations:

$$\frac{\partial U_N}{\partial\phi_i} = 0 \quad \forall i = 1,\ldots,N\ . \tag{S2}$$

In the case of bilayers, this set of equations reads

$$\begin{cases} -J\sin(\phi_1-\phi_2) + \mu_0 M_s H\sin\phi_1 = 0 \\ \ \ J\sin(\phi_1-\phi_2) + \mu_0 M_s H\sin\phi_2 = 0 \end{cases} \implies \begin{cases} -H_J/2\sin(\phi_1-\phi_2) + H\sin\phi_1 = 0 \\ \ \ H_J/2\sin(\phi_1-\phi_2) + H\sin\phi_2 = 0 \end{cases} \tag{S3}$$

where we have introduced the magnetic field scale $H_J = 2J/(\mu_0 M_s)$ associated with the inter-layer exchange coupling $J$. By summing the two equations we get the condition:

$$\sin\phi_1 + \sin\phi_2 = 2\sin\left(\frac{\phi_1+\phi_2}{2}\right)\cos\left(\frac{\phi_1-\phi_2}{2}\right) = 0 \qquad \implies \qquad \phi_1 = -\phi_2 \quad \text{or} \quad \phi_1 = \phi_2 + \pi\ . \tag{S4}$$

Among the two possible solutions, the first one has a lower energy at finite $H$, so we take $\phi_1 = -\phi_2 \equiv \phi$, where the angle $\phi$ satisfies

$$-H_J/2\sin(2\phi) + H\sin\phi = 0 \quad \implies \quad \sin\phi\,(H_J\cos\phi - H) = 0\ , \tag{S5}$$

whose solution is given by

$$\boxed{\phi = \phi_1 = -\phi_2 = \mathrm{Re}\left[\arccos\left(H/H_J\right)\right]\ .} \tag{S6}$$

We thus have that the magnetization in the two layers starts from a flopped configuration ($\phi_1 = \pi/2$, $\phi_2 = -\pi/2$) at $H = 0$, and then gradually cants in the direction of the field at $H \neq 0$, until the spin-flip transition occurs at $H = H_J$ and $\phi_1 = \phi_2 = 0$, i.e. both magnetizations are perfectly aligned with the external field. This is the solution represented in Fig. 3**a** of the main text.

We now consider the case of trilayers, for which the set of equations to be solved is:

$$\begin{cases} -H_J/2\sin(\phi_1-\phi_2) + H\sin\phi_1 = 0 \\ -H_J/2\sin(\phi_2-\phi_1) - H_J/2\sin(\phi_2-\phi_3) + H\sin\phi_2 = 0 \\ -H_J/2\sin(\phi_3-\phi_2) + H\sin\phi_3 = 0 \end{cases} \tag{S7}$$

By taking the difference between the first and the last equation we obtain the condition

$$\left[H_J\cos\left(\frac{\phi_1+\phi_3}{2} - \phi_2\right) - 2H\cos\left(\frac{\phi_1+\phi_3}{2}\right)\right]\sin\left(\frac{\phi_1-\phi_3}{2}\right) = 0\ , \tag{S8}$$

which, apart from a non-trivial solution that does not correspond to the lowest energy minimum, leads to $\phi_1 = \phi_3$, meaning that the outer layers share the same orientation. It is then convenient to introduce the relative angle $\theta$ between the magnetization of the central and outer layers, so that we can write $\phi_1 = \phi_3 = \phi$ and $\phi_2 = \phi + \theta$, and the equations become

$$\begin{cases} H_J/2\sin\theta + H\sin\phi = 0 \\ -H_J\sin\theta + H\sin(\phi+\theta) = 0 \end{cases} \implies \begin{cases} \sin\theta = -2H/H_J\sin\phi \\ \left[H_J - H\cos\phi\right]\sin\theta = H\sin\phi\cos\theta \end{cases}. \tag{S9}$$

By putting the two equations together, we thus obtain the following condition

$$\left[2 - 2H/H_J\cos\phi + \cos\theta\right]H\sin\phi = 0\ . \tag{S10}$$

In addition to the trivial solution $\phi = n\pi$ (with $n$ an integer), this leads to

$$\cos\theta = 2H/H_J \cos\phi - 2 \quad \Longrightarrow \quad 1 - \sin^2\theta = (2H/H_J \cos\phi - 2)^2 \tag{S11}$$

that with the help of Eq. (S9) can be written as an equation for $\phi$ only:

$$8H/H_J \cos\phi = 4(H/H_J)^2 + 3 \quad \Longrightarrow \quad \phi = \mathrm{Re}\left[\arccos\left(\frac{4H^2 + 3H_J^2}{8HH_J}\right)\right] \ . \tag{S12}$$

Replacing this result in Eq. (S11), we can obtain also the relative angle $\theta$

$$\cos\theta = (H/H_J)^2 - 5/4 \quad \Longrightarrow \quad \theta = \mathrm{Re}\left[\arccos\left(\frac{4H^2 - 5H_J^2}{4H_J^2}\right)\right] \tag{S13}$$

and, by expoiting Eq. (S9), the orientation of the central layer

$$\cos\phi_2 = \cos\phi\cos\theta - \sin\phi\sin\theta = \cos\phi\,(2H/H_J\cos\phi - 2) + 2H/H_J\sin^2\phi = 2H/H_J - 2\cos\phi = \frac{4H^2 - 3H_J^2}{4HH_J}$$

$$\Longrightarrow \quad \phi_2 = -\mathrm{Re}\left[\arccos\left(\frac{4H^2 - 3H_J^2}{4HH_J}\right)\right] \ . \tag{S14}$$

To summarise, in the case of trilayers we find

$$\boxed{\phi_1 = \phi_3 = \mathrm{Re}\left[\arccos\left(\frac{4H^2 + 3H_J^2}{8HH_J}\right)\right] \qquad \text{and} \qquad \phi_2 = -\mathrm{Re}\left[\arccos\left(\frac{4H^2 - 3H_J^2}{4HH_J}\right)\right] \ ,} \tag{S15}$$

which are the solutions depicted in Fig. 3**b** of the main text. At small fields, the arccos functions are imaginary, and the solution is simply $\phi_1 = \phi_3 = 0$ and $\phi_2 = \pi$. This simple collinear antiferromagnetic state (↑↓↑) is stable up to a critical field $H = H_J/2$ (spin-flop transition), at which non-trivial solutions become possible and the angles start to deviate from the field axis. By further increasing the field, the magnetization in each layer evolve in the direction of the field, until a perfect alignment ($\phi_1 = \phi_2 = \phi_3 = 0$) is reached at $H = 3H_J/2$ (spin-flop transition).

## Supplementary Note 4: Modelling the tunnelling conductance of multilayers

From band structure calculations within density-functional theory[6–8], it is known that in isolated monolayers of $CrCl_3$ the conduction band edge for majority spins is lower in energy than the minority-spin conduction band minimum. This results in a lower barrier eight for electrons tunnelling from graphite electrodes that have their spin parallel to the majority spins than for electrons with antiparallel spins, giving rise to a partial spin-filtering effect. The corresponding tunnelling amplitude matrix as a function of energy can be written as

$$t(E) = t_{\mathrm{P}}(E)\frac{\mathbb{1} + \hat{\boldsymbol{m}}\cdot\boldsymbol{\sigma}}{2} + t_{\mathrm{AP}}(E)\frac{\mathbb{1} - \hat{\boldsymbol{m}}\cdot\boldsymbol{\sigma}}{2} \tag{S16}$$

where $\sigma_i$ ($i = x, y, z$) are the spin-1/2 Pauli matrices, $\hat{\boldsymbol{m}}$ is the magnetization direction within the layer, and $t_{\mathrm{P/AP}}(E)$ is the tunnelling amplitude for electrons with spin parallel/antiparallel to the magnetization direction. In the linear transport regime, the conductance at low temperature is then given by

$$G_{\mathrm{mono}}/G_0 = \mathrm{Tr}\left[t^\dagger(E_{\mathrm{F}})t(E_{\mathrm{F}})\right] = |t_{\mathrm{P}}(E_{\mathrm{F}})|^2 + |t_{\mathrm{AP}}(E_{\mathrm{F}})|^2 \tag{S17}$$

where $E_{\mathrm{F}}$ is the Fermi energy in the graphite electrodes and $G_0$ is a conductance unit (that depends on the density of states at the Fermi energy).

To compute the tunnelling conductance of $CrCl_3$ multilayers, we need to combine the spin-filtering behaviour discussed above from each layer, taking into account that the orientation of the magnetization can be different within each layer. Simple analytical expressions can be obtained in the limit when the transmission amplitude matrix through a multilayer can be expressed as the product of transmission amplitude matrices $t_i$ from each layer, where each $t_i$ has the same expression as in Eq. (S16) with $\hat{\boldsymbol{m}}$ oriented according to the magnetization of the $i$-th layer. In this way, $t_{\mathrm{bi}} = t_1 \cdot t_2$ for the bilayer and $t_{\mathrm{tri}} = t_1 \cdot t_2 \cdot t_3$ for the trilayer. Reminding that in the case of trilayers the external layers share the same magnetization direction, the transmission amplitude matrix can be expressed as a function of a

single relative angle $\theta$ both for bi- and trilayers, corresponding to the relative angle between the two layers in bilayers and the angle between the internal and external layers in trilayers. The conductance can be then obtained as

$$G_{\mathrm{bi/tri}}(\theta)/G_0 = \mathrm{Tr}\left[t^{\dagger}_{\mathrm{bi/tri}}(\theta)t_{\mathrm{bi/tri}}(\theta)\right] \ , \tag{S18}$$

giving rise to

$$G_{\mathrm{bi}}(\theta)/G_0 = \frac{(a+b)^2}{2} + \frac{(a-b)^2}{2}\cos\theta \tag{S19}$$

for bilayers and

$$G_{\mathrm{tri}}(\theta)/G_0 = \frac{(a+b)^3 + c(a-b)^2}{4} + \frac{(a-b)^2(a+b)}{2}\cos\theta + \frac{(a-b)^2(a+b-c)}{4}\cos^2\theta \tag{S20}$$

for trilayers, where we have introduced the following shorthand notation:

$$a = |t_{\mathrm{P}}(E_{\mathrm{F}})|^2 \qquad b = |t_{\mathrm{AP}}(E_{\mathrm{F}})|^2 \qquad c = t_{\mathrm{P}}(E_{\mathrm{F}})t^*_{\mathrm{AP}}(E_{\mathrm{F}}) + t_{\mathrm{AP}}(E_{\mathrm{F}})t^*_{\mathrm{P}}(E_{\mathrm{F}}) \ . \tag{S21}$$

These results can be translated into a magnetoconductance (i.e. a conductance versus applied magnetic field) $G(H)$ by combining the above expression with the information on the evolution of the relative angle $\theta(H)$ between the magnetization in adjacent layers from the antiferromagnetic linear-chain model (see Supplementary Note 3). The parameters $a$, $b$, and $c$ in Eqs. (S19)-(S20) can be tuned to reproduce the experimental results, as show in Fig. 3 of the main text.

These simplified expressions can be justified more rigorously by modelling each layer as a rectangular potential barrier with height $V_{\mathrm{P/AP}}$ for spins parallel/antiparallel to the magnetization, so that the transmission amplitudes read:

$$t_{\mathrm{P/AP}}(E) = \frac{1}{\cosh\left[d\sqrt{2m^*(V_{\mathrm{P/AP}}-E)/\hbar^2}\right] + i\frac{V_{\mathrm{P/AP}}-2E}{2\sqrt{E(V_{\mathrm{P/AP}}-E)}}\sinh\left[d\sqrt{2m^*(V_{\mathrm{P/AP}}-E)/\hbar^2}\right]} \qquad \text{with} \quad V_{\mathrm{P/AP}} > E \tag{S22}$$

where $d$ is the monolayer thickness and $m^*$ is an effective mass (assumed for simplicity to be the same throughout the system). The conductance of a monolayer is then given by

$$G_{\mathrm{mono}}/G_0 = \frac{1}{1+\frac{V_{\mathrm{P}}^2\sinh^2\left[d\sqrt{2m^*(V_{\mathrm{P}}-E)/\hbar^2}\right]}{4E(V_{\mathrm{P}}-E)}} + \frac{1}{1+\frac{V_{\mathrm{AP}}^2\sinh^2\left[d\sqrt{2m^*(V_{\mathrm{AP}}-E)/\hbar^2}\right]}{4E(V_{\mathrm{AP}}-E)}} \ . \tag{S23}$$

This approach can be generalized to any number of layers $N$ by modelling the multilayer as a step-wise potential barrier with overall thickness $Nd$. Within a single layer the barrier height is simply $V_{\mathrm{P/AP}}$ for spins parallel/antiparallel to the magnetization, although the definition of parallel/antiparallel depends on the local orientation of the magnetization. In order to obtain the overall transmission, we use a transfer-matrix approach, decomposing the full transfer matrix into a product of simple transfer matrices corresponding to:

- the transfer matrix from the potential barrier to the (right) electrode –defined up to a factor which is canceled out when combining it with its inverse corresponding to the transfer from the left electrode to the barrier–, defined in the basis of the local spin orientation

$$D = \frac{1}{2}\begin{pmatrix} 1+i\kappa & 0 & 1-i\kappa & 0 \\ 0 & \frac{1+i\alpha\kappa}{\sqrt{\alpha}} & 0 & \frac{1-i\alpha\kappa}{\sqrt{\alpha}} \\ 1-i\kappa & 0 & 1+i\kappa & 0 \\ 0 & \frac{1-i\alpha\kappa}{\sqrt{\alpha}} & 0 & \frac{1+i\alpha\kappa}{\sqrt{\alpha}} \end{pmatrix} \tag{S24}$$

- the transfer matrix corresponding to the plain propagation within the barrier, in the basis of the local spin orientation

$$P = \begin{pmatrix} e^{-\kappa l} & 0 & 0 & 0 \\ 0 & e^{-\kappa\alpha l} & 0 & 0 \\ 0 & 0 & e^{\kappa l} & 0 \\ 0 & 0 & 0 & e^{\kappa\alpha l} \end{pmatrix} \tag{S25}$$

- the transfer matrix between one layer and the next, assuming a rotation of the magnetization by an angle $\theta$ in the plane of the layers:

$$R(\theta) = \begin{pmatrix} \cos\left(\frac{\theta}{2}\right) & \frac{\alpha+1}{2\sqrt{\alpha}}\sin\left(\frac{\theta}{2}\right) & 0 & \frac{1-\alpha}{2\sqrt{\alpha}}\sin\left(\frac{\theta}{2}\right) \\ -\frac{\alpha+1}{2\sqrt{\alpha}}\sin\left(\frac{\theta}{2}\right) & \cos\left(\frac{\theta}{2}\right) & \frac{1-\alpha}{2\sqrt{\alpha}}\sin\left(\frac{\theta}{2}\right) & 0 \\ 0 & \frac{1-\alpha}{2\sqrt{\alpha}}\sin\left(\frac{\theta}{2}\right) & \cos\left(\frac{\theta}{2}\right) & \frac{\alpha+1}{2\sqrt{\alpha}}\sin\left(\frac{\theta}{2}\right) \\ \frac{1-\alpha\sin}{2\sqrt{\alpha}}\left(\frac{\theta}{2}\right) & 0 & -\frac{\alpha+1}{2\sqrt{\alpha}}\sin\left(\frac{\theta}{2}\right) & \cos\left(\frac{\theta}{2}\right) \end{pmatrix} \tag{S26}$$

where

$$\kappa = \sqrt{\frac{V_\mathrm{P} - E}{E}} \qquad \alpha = \sqrt{\frac{V_\mathrm{AP} - E}{V_\mathrm{P} - E}} \qquad l = \frac{\sqrt{2m^* E}}{\hbar} d \tag{S27}$$

In this way the overall transfer matrices of mono-, bi-, and tri-layers are given respectively by (in the spin basis of the first layer)

$$M_\mathrm{mono} = DPD^{-1} \qquad M_\mathrm{bi}(\theta) = U(\theta)DPR(\theta)PD^{-1} \qquad M_\mathrm{tri}(\theta) = DPR(\theta)PR(-\theta)PD^{-1} \tag{S28}$$

where we have exploited the fact that in trilayers the magnetization orientation in the outer layers is identical and we introduced a final change of basis in the case of bilayers, defined through

$$U(\theta) = \begin{pmatrix} \cos\left(\frac{\theta}{2}\right) & \sin\left(\frac{\theta}{2}\right) & 0 & 0 \\ -\sin\left(\frac{\theta}{2}\right) & \cos\left(\frac{\theta}{2}\right) & 0 & 0 \\ 0 & 0 & \cos\left(\frac{\theta}{2}\right) & \sin\left(\frac{\theta}{2}\right) \\ 0 & 0 & -\sin\left(\frac{\theta}{2}\right) & \cos\left(\frac{\theta}{2}\right) \end{pmatrix} \tag{S29}$$

The transfer matrices are $4 \times 4$ matrices that can be written in block form as

$$M_i = \begin{pmatrix} [M_i]_{11} & [M_i]_{12} \\ [M_i]_{21} & [M_i]_{22} \end{pmatrix} \tag{S30}$$

where $[M_i]_{k\ell}$ are $2 \times 2$ blocks and that respect the following conditions

$$\det M_i = 1 \quad \text{and} \quad M_i^\dagger \Sigma_z M_i = \Sigma_z \ , \qquad \text{with} \quad \Sigma_z = \begin{pmatrix} 1 & 0 & 0 & 0 \\ 0 & 1 & 0 & 0 \\ 0 & 0 & -1 & 0 \\ 0 & 0 & 0 & -1 \end{pmatrix} . \tag{S31}$$

Once the overall transfer matrix is computed, the transmission amplitude can be obtained by inverting the lower-right block as $t_i = [M_i]_{22}^{-1}$. In the case of monolayers, the transmission matrix can be computed analytically, resulting in

$$t_\mathrm{mono} = \begin{pmatrix} t_\mathrm{P} & 0 \\ 0 & t_\mathrm{AP} \end{pmatrix} = \begin{pmatrix} \frac{1}{\cosh(\kappa l) + i\frac{\kappa^2-1}{2\kappa}\sinh(\kappa l)} & 0 \\ 0 & \frac{1}{\cosh(\kappa l\alpha) + i\frac{\kappa^2\alpha^2-1}{2\kappa\alpha}\sinh(\kappa\alpha l)} \end{pmatrix} \tag{S32}$$

which is equivalent to Eq. (S22) upon substituting the definitions (S27).

In the case of bi- and trilayers compact analytical expressions are not easily achievable, apart from special limiting cases such as the configuration with parallel magnetization in all layers, when:

$$t_\mathrm{bi/tri}(\theta = 0) = \begin{pmatrix} \frac{1}{\cosh(N\kappa l) + i\frac{\kappa^2-1}{2\kappa}\sinh(N\kappa l)} & 0 \\ 0 & \frac{1}{\cosh(N\kappa l\alpha) + i\frac{\kappa^2\alpha^2-1}{2\kappa\alpha}\sinh(N\kappa\alpha l)} \end{pmatrix} \quad \text{with} \quad N = 2, 3 \text{ respectively} \tag{S33}$$

which correctly corresponds to a uniform rectangular barrier with thickness $Nd$.

The conductance of bi- and trilayers can be obtained by replacing the transmission amplitude matrices $t_\mathrm{bi/tri}(\theta)$ in Eq. (S18). A good agreement with experiment is obtained by tuning the parameters $\kappa$, $\alpha$, and $l$ entering the expression for $G$. The corresponding angular dependence can be expanded in series of $\cos\theta$, resulting in the following leading contributions that agree with the simplified expressions in Eqs. (S19)-(S20):

$$G_\mathrm{bi}(\theta)/G_\mathrm{max} = 0.810 + 0.188\cos\theta + \ldots \tag{S34}$$

and

$$G_\mathrm{tri}(\theta)/G_\mathrm{max} = 0.713 + 0.266\cos\theta + 0.020\cos^2\theta + \ldots \ . \tag{S35}$$

## Supplementary Note 5: Thickness evolution of the spin-flip and spin-flop transition fields

The spin-flip and spin-flop transition fields denote the stability boundary of the simple collinear ferromagnetic and antiferromagnetic solution to Eq. (S2), respectively. Indeed, denoting with $\phi_i$ the angle formed by the magnetization the $i$-th layer with the magnetic field direction, the spin-flip field is defined as the minimum field at which the ferromagnetic solution $\phi_1 = \phi_2 = \cdots = \phi_N = 0$ starts to be stable, while the spin-flop field is the maximum field at which the antiferromagnetic solution $\phi_{2i+1} = 0$ and $\phi_{2i} = \pi$ can be considered stable. Stability means that small deviations in the angles $\phi_i$ lead to an increase in energy, so that the system is favoured to remain in the collinear solution. This corresponds to saying that, in order to be stable, a solution $\{\phi_i^s\}_{i=1,\ldots,N}$ to Eq. (S2) also has to be a minimum of the magnetic energy $U_N$, i.e. that the matrix of second derivatives of $U_N$ has to be positive definite:

$$\det(A^s) > 0 \qquad \text{with} \qquad A^s_{ij} = \left.\frac{\partial^2 U_N}{\partial\phi_i\partial\phi_j}\right|_{\phi_i=\phi_i^s} . \tag{S36}$$

A stable solution ($\det(A^s) > 0$) becomes unstable ($\det(A^s) < 0$) as a function of the field by passing through a critical value at which $\det(A^s) = 0$. The stability boundary can thus be obtained by imposing the condition $\det(A^s) = \prod_{k=1}^N \lambda_k^s = 0$ for a given solution, i.e. by looking for the critical field at which at least one of the eigenvalues $\lambda_k^s$ of $A^s$ vanishes.

We start by considering the collinear ferromagnetic solution $\phi_1^{\rm FM} = \phi_2^{\rm FM} = \cdots = \phi_N^{\rm FM} = 0$ when the magnetic field is applied in-plane. By taking the second derivatives of $U_N$ in Eq. (S1), we find that the matrix $A^{\rm FM}$ has a tridiagonal form and reads

$$A^{\rm FM} = \begin{pmatrix} H - H_J/2 & H_J/2 & & & & 0 \\ H_J/2 & H - H_J & H_J/2 & & & \\ & H_J & \ddots & \ddots & & \\ & & \ddots & \ddots & H_J/2 & \\ & & & H_J/2 & H - H_J & H_J/2 \\ 0 & & & & H_J/2 & H - H_J/2 \end{pmatrix} . \tag{S37}$$

Using standard approaches for tridiagonal matrices, it is straightforward to obtain the following set of eigenvalues for a generic number of layers $N$:

$$\lambda_k^{\rm FM} = H - H_J + H_J \cos\left(\frac{k\pi}{N}\right) \qquad \text{with} \quad k = 1, \ldots, N-1 . \tag{S38}$$

We then see that for sufficiently high fields all eigenvalues are positive and the collinear antiferromagnetic state is thus stable. By decreasing $H$, the stability breaks down when the smallest eigenvalue (corresponding to $k = N-1$) vanishes and the matrix $A^{\rm FM}$ is no longer positive definite. This leads to the following condition for the spin-flip field $H_2^{\parallel}$ in parallel configuration:

$$H_2^{\parallel} - H_J + H_J \cos\left(\frac{N-1}{N}\pi\right) = 0 \quad \Longrightarrow \quad H_2^{\parallel} = H_J + H_J \cos\left(\frac{\pi}{N}\right) = 2H_J \cos^2\left(\frac{\pi}{2N}\right) . \tag{S39}$$

When the field is applied perpendicular to the layers, the matrix of second derivatives simply acquires an additional contribution proportional to the identity matrix, $A^{\rm FM} \to A^{\rm FM} + K_\perp/(\mu_0 M_s)\mathbb{1}$, and the spin-flip field is shifted by a constant independent of the number of layers:

$$H_2^{\perp} = 2H_J \cos^2\left(\frac{\pi}{2N}\right) + K_\perp/(\mu_0 M_s) = 2H_J \cos^2\left(\frac{\pi}{2N}\right) + M_s/V \tag{S40}$$

where we have exploited the fact that the easy-plane magnetic anisotropy $K_\perp$ is dominated by magnetostatic contributions so that $K_\perp = \mu_0 M_s^2/V$. We thus have that, as reported in the main text, the spin-flip field in parallel and perpendicular configuration evolves with the number of layers $N$ as follows:

$$\boxed{H_2^{\parallel}(N) = 2H_J \cos^2\left(\frac{\pi}{2N}\right) \qquad H_2^{\perp}(N) = 2H_J \cos^2\left(\frac{\pi}{2N}\right) + M_s/V .} \tag{S41}$$

We now consider the collinear antiferromagnetic state in parallel field, corresponding to the solution $\phi_{2i+1}^{\rm AF} = 0$ and $\phi_{2i}^{\rm AF} = \pi$ to Eq. (S2). We find that also in this case the matrix of second derivatives is tridiagonal, although it is

different for even-$N$ and odd-$N$ multilayers (notice the different signs with which the magnetic field $H$ is appearing in the extremal diagonal elements):

$$A^{\rm AF}_{\rm even} = \begin{pmatrix} H_J/2+H & -H_J/2 & & & & 0 \\ -H_J/2 & H_J-H & H_J/2 & & & \\ & -H_J & \ddots & \ddots & & \\ & & \ddots & \ddots & -H_J/2 & \\ & & & -H_J/2 & H_J+H & -H_J/2 \\ 0 & & & & -H_J/2 & H_J/2-H \end{pmatrix} . \tag{S42}$$

$$A^{\rm AF}_{\rm odd} = \begin{pmatrix} H_J/2+H & -H_J/2 & & & & 0 \\ -H_J/2 & H_J-H & H_J/2 & & & \\ & -H_J & \ddots & \ddots & & \\ & & \ddots & \ddots & -H_J/2 & \\ & & & -H_J/2 & H_J-H & -H_J/2 \\ 0 & & & & -H_J/2 & H_J/2+H \end{pmatrix} . \tag{S43}$$

Using linear algebra techniques, we can prove that in both cases the eigenvalues take the general form

$$\lambda^{\rm AF}_{\pm} = H_J \pm \sqrt{H^2 + H_J^2 \left(\frac{z+z^{-1}}{2}\right)^2} \tag{S44}$$

where $z$ satisfies

$$\begin{cases} (1-cz)(1-cz^{-1})(z^N - z^{-N}) = 0 & \text{for } N \text{ even} \\ \left[4c - (c^2+1)(z+z^{-1})\right](z^N - z^{-N}) + (c^2-1)(z-z^{-1})(z^N+z^{-N}) = 0 & \text{for } N \text{ odd} \end{cases} \quad \text{with} \quad c = \sqrt{\frac{H_J-\lambda-H}{H_J-\lambda+H}} \tag{S45}$$

For even-$N$ multilayers, the corresponding equation can be solved, giving rise to the following set of $N$ eigenvalues:

$$\lambda^{\rm AF,even}_{0,\pm} = H_J/2 \pm \sqrt{H^2 + H_J^2/4} \qquad \lambda^{\rm AF,even}_{k,\pm} = H_J \pm \sqrt{H^2 + H_J^2 \cos^2\left(\frac{k\pi}{N}\right)} \quad \text{with} \quad k = 1, \ldots, N/2-1 \tag{S46}$$

In particular, we see that the lowest eigenvalue $\lambda^{\rm AF,even}_{0,-} = H_J/2 - \sqrt{H^2+H_J^2/4}$ vanishes for $H=0$ and it is negative for $H \neq 0$. This means that in even-$N$ multilayers the spin-flop transition occurs at zero field ($H_1 = 0$), and the collinear antiferromagnetic state is unstable at any finite magnetic field.

In the case of odd-$N$ multilayers, a closed-form analytical expression for the eigenvalues is not easily achievable. Still, we can determine the spin-flop field $H_1$ from the condition that one of the eigenvalues vanishes:

$$\lambda^{\rm AF,odd}_{-} = 0 \qquad \Longrightarrow \qquad H^2 = H_J^2 \left[1 - \left(\frac{z+z^{-1}}{2}\right)^2\right] . \tag{S47}$$

Putting this expression into Eq. (S45), we obtain the consistency condition

$$(z^N + z^{-N}) = 0 \qquad \Longrightarrow \qquad z_k = e^{i\frac{2k+1}{2N}\pi} \qquad \Longrightarrow \qquad H_k = H_J \sin\left(\frac{2k+1}{2N}\pi\right) \quad \text{with} \quad k = 0, \ldots, \frac{N-3}{2} \tag{S48}$$

We thus have that the minimum field at which one of the eigenvalues vanishes and becomes negative corresponds to $k=0$. This means that in a odd-$N$ multilayer the collinear antiferromagnetic state becomes unstable above the following spin-flop field:

$$\boxed{H_1(N) = H_J \sin\left(\frac{\pi}{2N}\right) ,} \tag{S49}$$

which is the thickness evolution reported in the main text.

We finally mention that at finite temperature the energy (see Methods) can be simply written:

$$U_N(T) = J\left[\frac{M(T)}{M_s}\right]^2 \sum_{i=1}^{N-1} \cos(\phi_i - \cos\phi_{i+1}) - \mu_0 M_s H \frac{M(T)}{M_s} \sum_{i=1}^{N} \cos\phi_1 \ . \tag{S50}$$

where we considered for definiteness the field to be applied parallel to the layers. We thus see that this expression can be obtained from the zero-temperature form in Eq. (S1) by replacing:

$$J \to J\left[\frac{M(T)}{M_s}\right]^2 \qquad H \to H\left[\frac{M(T)}{M_s}\right] \qquad \left(\text{and similarly} \quad K_\perp \to K_\perp\left[\frac{M(T)}{M_s}\right]^2\right) \tag{S51}$$

The same mapping can be then applied to obtain the transition fields at finite temperature:

$$\begin{gathered} H_1(N,T) = H_J \frac{M(T)}{M_s} \sin\left(\frac{\pi}{2N}\right) \ , \qquad H_2^{\parallel}(N,T) = 2H_J \frac{M(T)}{M_s} \cos^2\left(\frac{\pi}{2N}\right) \ , \\ H_2^{\perp}(N,T) = 2H_J \frac{M(T)}{M_s} \cos^2\left(\frac{\pi}{2N}\right) + M(T)/V \ . \end{gathered} \tag{S52}$$

From these expressions one can derive the scaling relationships that we discuss in the main text:

$$\boxed{\frac{H_2^{\parallel}(N,T)}{H_J} = 2\cos^2\left(\frac{\pi}{2N}\right) \frac{M(T)}{M_s} \ , \qquad \frac{H_1(N,T)}{H_2^{\parallel}(N,T)} = \frac{\sin\left(\frac{\pi}{2N}\right)}{2\cos^2\left(\frac{\pi}{2N}\right)} \ .} \tag{S53}$$

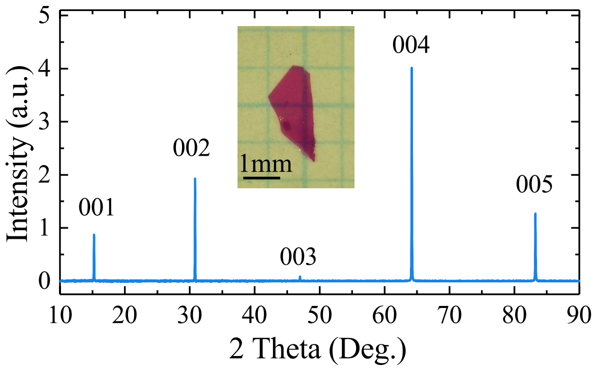


**Supplementary Fig.** 1. **Crystal structure of bulk $CrCl_3$.** X-ray diffraction pattern from the cleavage plane of a $CrCl_3$ crystal. The platelike crystal is shown in the inset. Only the reflections *[00l]* are present, proving that crystals cleave in the ab-plane of the C12/m structure.

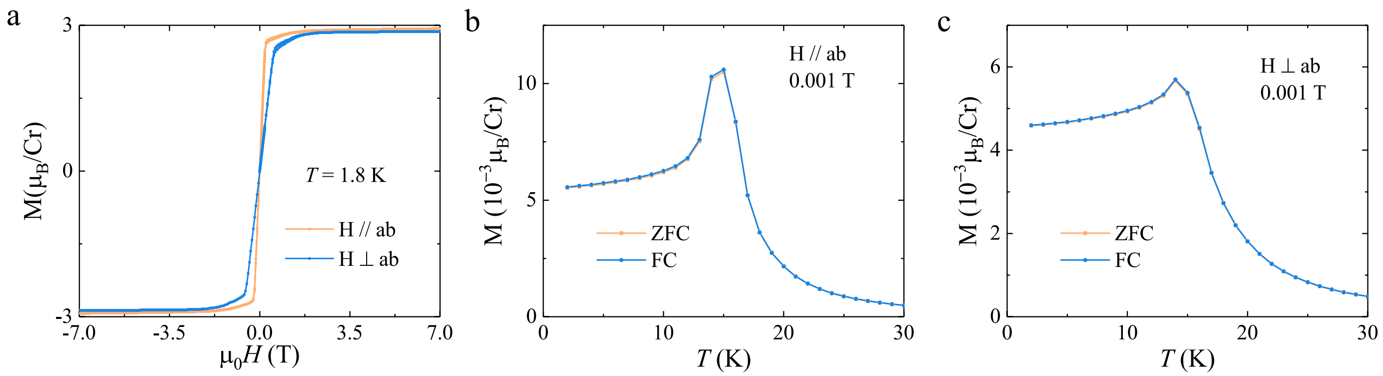


**Supplementary Fig.** 2. **Magnetism of bulk $CrCl_3$.** (a) Isothermal magnetization of a $CrCl_3$ crystal measured at 1.8 K for two orientations of the applied magnetic field, either parallel (blue line) or perpendicular (orange line) to the cleavage ab-plane. (b) and (c) Magnetic moment of $CrCl_3$ as a function of temperature at low magnetic field ($\mu_0 H = 1\,\mathrm{mT}$) applied either parallel (b) or perpendicular (c) to cleavage ab-plane. These curves show the anisotropic magnetic response of $CrCl_3$ crystals and the magnetic transition.

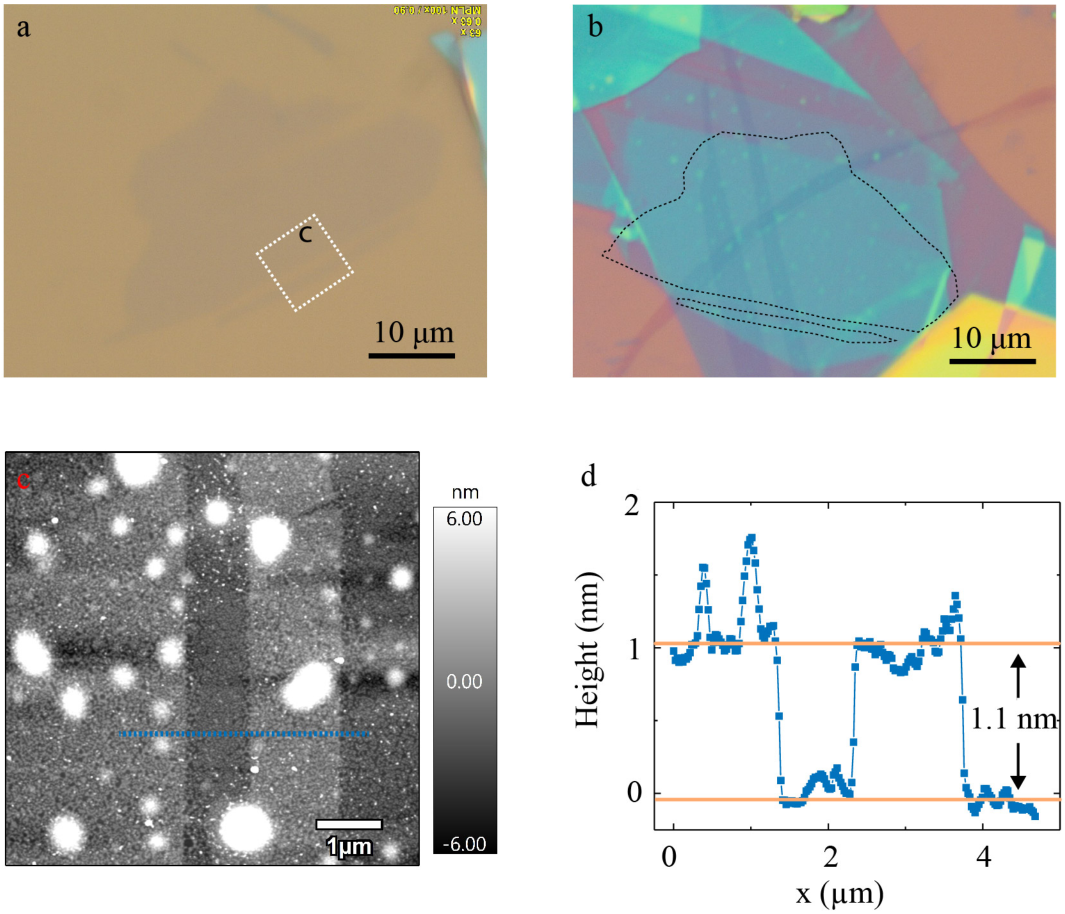


**Supplementary Fig.** 3. **$CrCl_3$ bilayer.** (a): optical microscope image of a bilayer $CrCl_3$ exfoliated onto a silicon substrate covered with 90 nm of silicon oxide. (b): optical microscope image of a multilayer graphene/bilayer $CrCl_3$/multilayer graphene junction encapsulated in between two hBN crystals. The black dots outline the contour of the $CrCl_3$ layer, not easily visible after encapsulation. The microscope images shown in (a) and (b) have been taken inside the glove box used to assemble the device. (c): Atomic force microscope image of the device after encapsulation. The imaged part of the $CrCl_3$ flake corresponds to the area inside the dotted white line shown in panel (a). (d): Height profile of the $CrCl_3$ bilayer measured along the dotted blue line in panel (c). The step height indicates that the $CrCl_3$ is indeed a bilayer (as the interlayer distance extracted from the profile is the expected one, i.e. 0.58 nm).

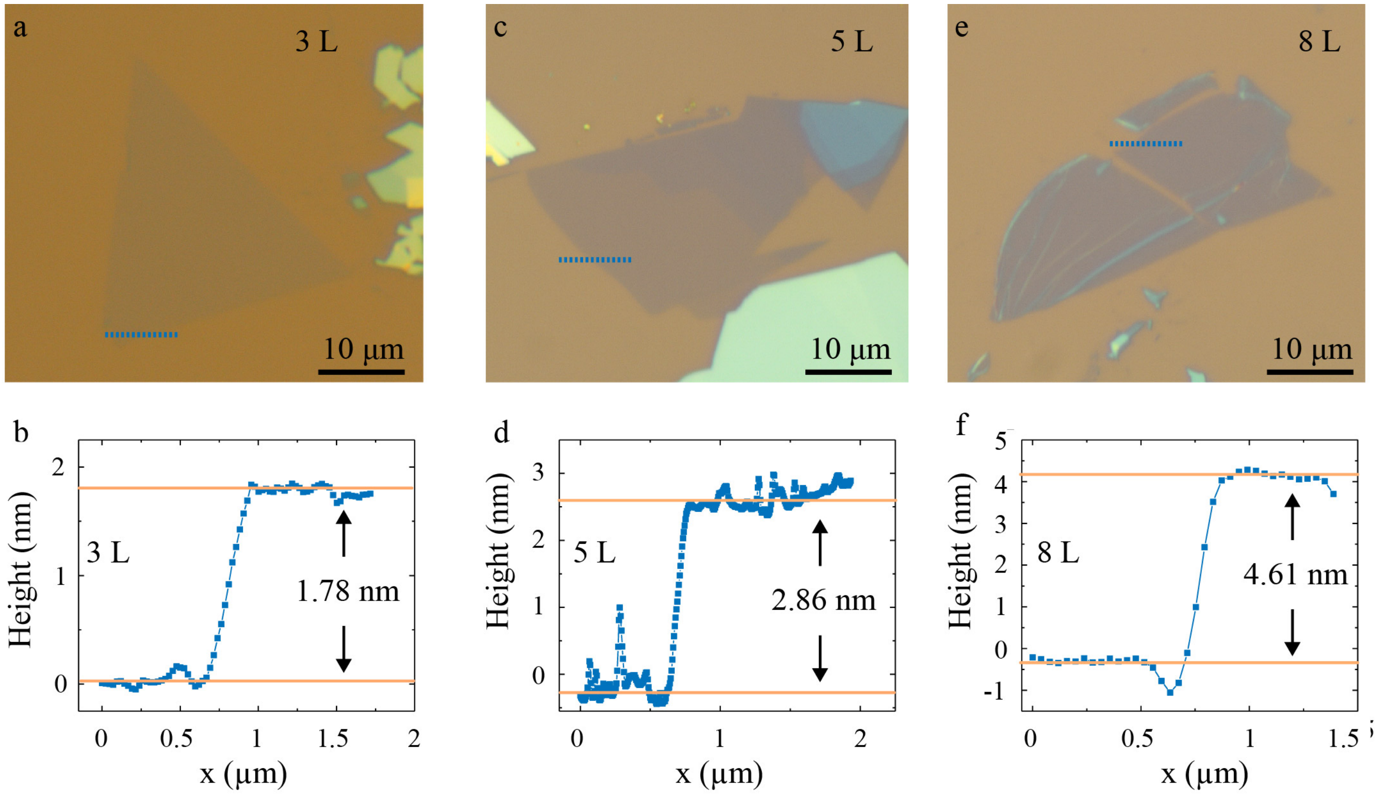


**Supplementary Fig.** 4. **$CrCl_3$ multilayers.** Optical microscope images of different $CrCl_3$ multilayers exfoliated on Si substrates covered with 90 nm $SiO_2$ and corresponding height profiles measured with an atomic force microscope. The optical microscope images are taken inside the glove box used to assemble the devices, whereas the atomic force measurements are taken outside, after encapsulation. For each multilayer, the height profile is measured along the dotted blue line shown in the corresponding optical microscope image. As we infer from the value of the step in the height profile, panels (a) and (b) correspond to a $CrCl_3$ trilayer, (c) and (d) to a $CrCl_3$ five-layer sample, and (e) and (f) to a $CrCl_3$ eight-layer.

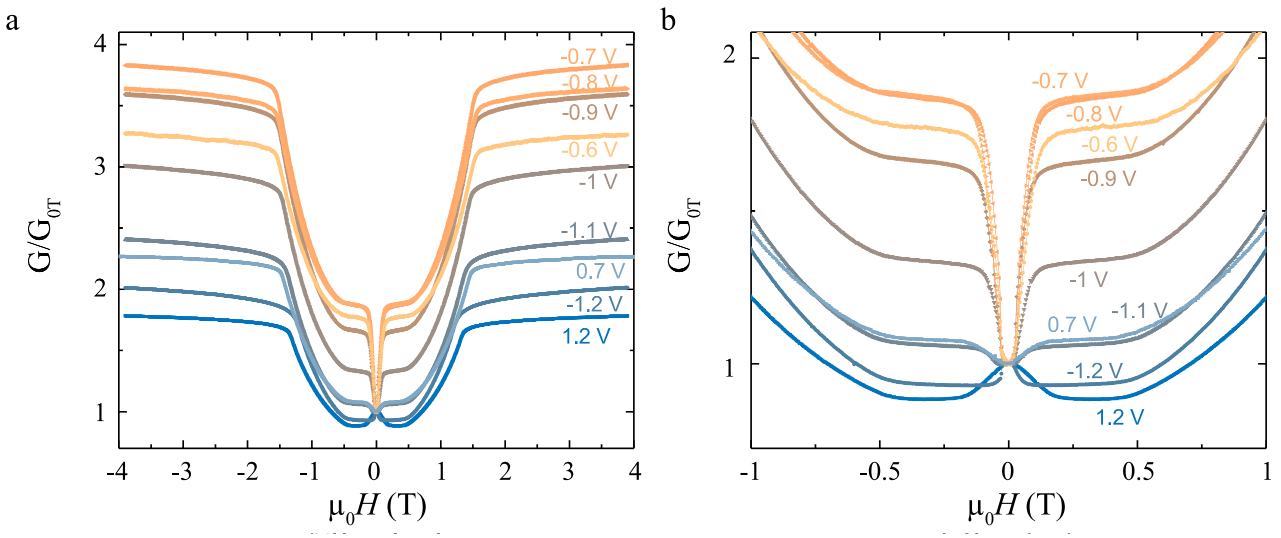


**Supplementary Fig.** 5. **Low-field magnetoconductance of odd-$N$ multilayers.** Odd-$N$ multilayers exhibit a small feature in their tunnelling magnetoconductance that appears at low field, i.e., values of $H$ that –for sufficiently small $N$– are smaller than the magnetic field $H_1$ at which the spin-flop transition occurs. As we discussed in the main text, this low-field feature is strongly sample and bias dependent. Here we illustrate the bias dependence with magnetoconductance data taken on a trilayer $CrCl_3$ device. Panel (a) and (b) show the tunnelling magnetoconductance (normalized to the $H = 0$ value) measured at the applied bias indicated next to the corresponding curves. In (a) the magnetoconductance curves are shown over a large magnetic field range, to illustrate that the overall behavior at the spin-flip and spin-flop transition does not depend on the applied bias. In (b) the same data are plotted in a smaller $H$ range to put in evidence the very strong bias dependence of the feature at low field (already visible in (a)). This feature typically manifests itself as a dip in conductance, but for specific values of bias the magnetoconductance dip can be turned into a peak. The origin of the phenomenon, as well as the reason for the strong bias dependence, are not currently understood.

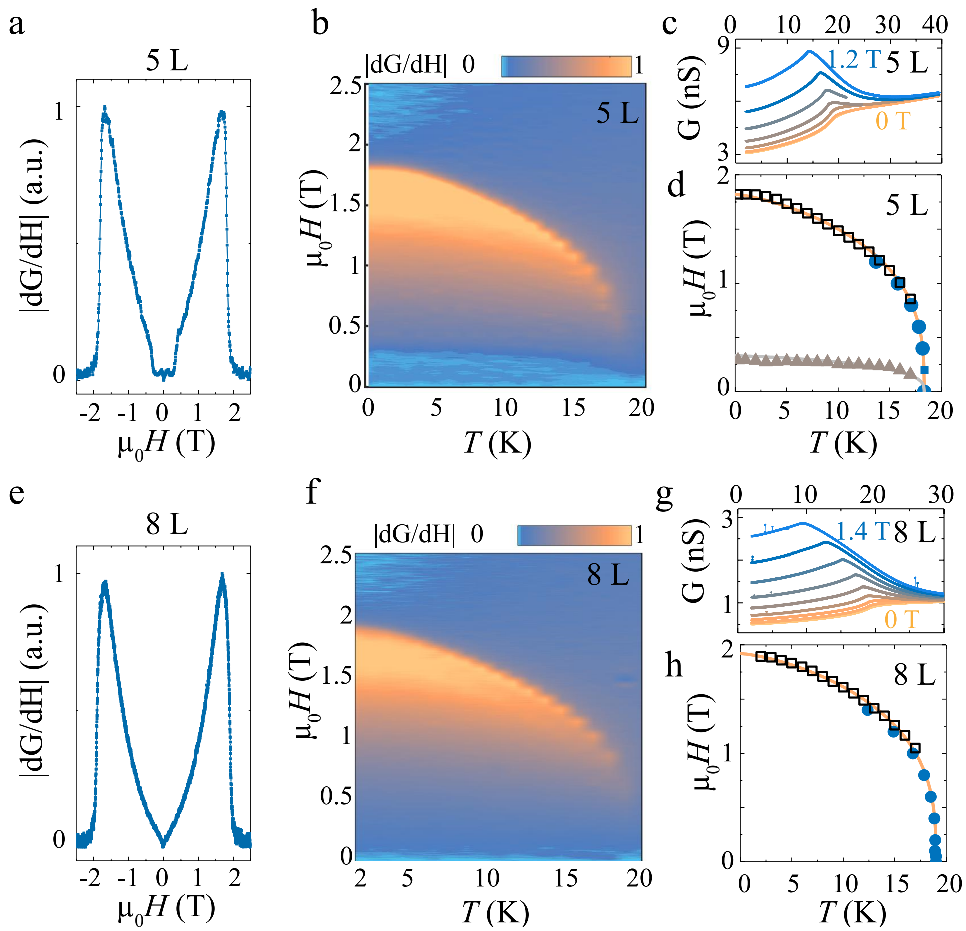


**Supplementary Fig.** 6. **Phase diagram of thicker $CrCl_3$ multilayers.** In the main text we have shown $dG/dH$ data for bi and trilayer $CrCl_3$ as a function of $H$ and $T$. We have used that data to discuss similarities (e.g., the presence of the spin-flip transition) and differences (e.g., the presence or absence of a spin-flop transition at finite $H$) of even and odd-$N$ $CrCl_3$ mutlilayers, and to determine the magnetic phase boundaries present in these systems. Here we show analogous data for another odd-$N$ ($N = 5$) and another even-$N$ ($N = 8$) multilayer (see panels (a-d) for $N = 5$ and panels (e-h) for $N = 8$). (a): $H$ dependence of $dG/dH$ measured at 250 mK on a $N = 5$ multilayer. Note the extended $H$ interval around $H = 0$ over which $dG/dH$ (nearly) vanishes. We take the value of $H$ at the end of this interval as a measure of $H_1$ (see also Fig. S9). At higher field, the value of $H$ at which $dG/dH$ jumps down to $dG/dH \simeq 0$ corresponds to $H_2$. (b): Colour plot of $dG/dH$ measured on a $N = 5$ multilayer, showing the full evolution of the tunnelling magnetoconductance with $H$ and $T$, from which we track the evolution of $H_1(T)$ and of $H_2(T)$. (c): conductance of a $N = 5$ multilayer measured as a function of $T$ for different values of in-plane applied magnetic field (from 0 T to 1.2 T, in steps of 0.2 T). (d): Phase boundaries of a $N = 5$ multilayer extracted from the data shown in panels (b) and (c), indicating the presence of both a finite-$H$ spin-flop transition, and of a spin-flip transition at higher field. Panels (e-h) show data measured on a $N = 8$ multilayer that correspond to the data shown in panels (a-d) for the $N = 5$ multilayer. As a key difference, note that in the $N = 8$ multilayer $dG/dH$ starts increasing monotonously from $H = 0$ (see panel (e)), as there is no finite $H$ spin-flop transition in even-$N$ multilayers. As a result only one phase boundary is visible in panel (h).

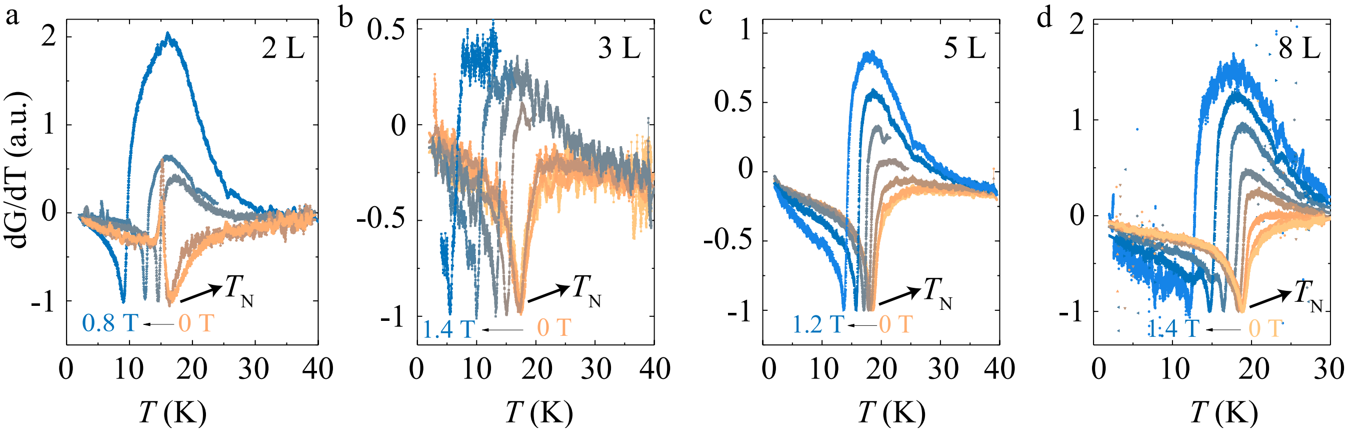


**Supplementary Fig.** 7. **Identification of the critical temperature**. In Fig. 2(e) and 2(g) of the main text, as well as in Fig. S6(c) and S6(g) of the supplementary material we have shown the $T$ dependence of the conductance measured for different values of applied magnetic field $H$, from which we can extract the critical temperature of our $CrCl_3$ multilayers. In practice, to determine the critical temperature, additional sensitivity is gained by looking at $dG/dT$ (rather than at $G(T)$). That is why in panels (a-d) we show $dG/dT$ data at different values of applied in-plane magnetic field (0.2 T per step) respectively for $N = 2, 3, 5$ and 8 multilayers. $dG/dT$ data are normalized to the value of minimum $dG/dT$ (i.e., to the value of $dG/dT$ at the position of the dip), which corresponds to the critical temperature $T_N$.

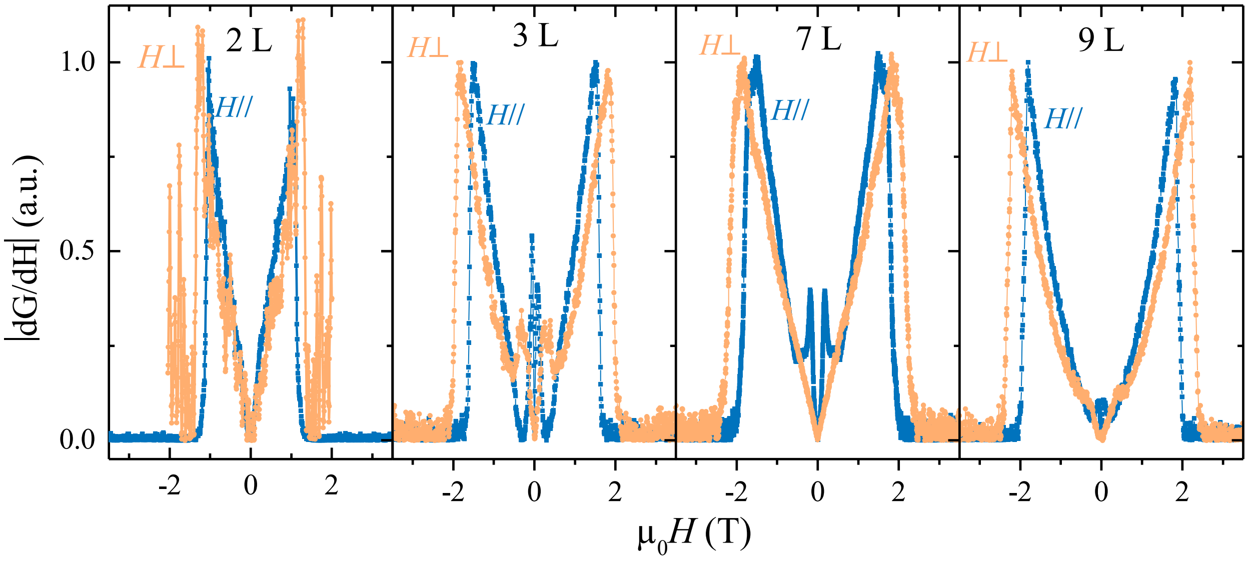


**Supplementary Fig.** 8. **Comparison of $dG/dH$ data as a function of in-plane and perpendicular magnetic field.** As we discussed in the main text, the spin-flip transition is observed to occur in all multilayers at a field value $H = H_2$ that depends on whether the field is applied parallel ($H_2^{\parallel}$) or perpendicular ($H_2^{\perp}$) to the $CrCl_3$ layers. The difference $H_2^{\perp} - H_2^{\parallel}$ is found to be the same for all devices, irrespective of multilayer thickness ($H_2^{\perp} - H_2^{\parallel} \simeq 0.35$ T). From this observation we infer that the magnetic anisotropy in $CrCl_3$ is dominated by shape anistropy. Panels (a-d) show data measured on $N = 2, 3, 7$ and 9 multilayers on which this conclusion is based (together with the data shown in the main text for $N = 5$ and $N = 8$). In panel (a), high field data on the bilayer devices has been removed, due to the presence of oscillations originating from the formation of Landau levels in the graphene contacts (these oscillations are not visible in devices based on thicker $CrCl_3$ multilayers, likely because the much higher tunneling resistance of those devices requires the application of much larger bias to perform the magnetoconductance measurements).

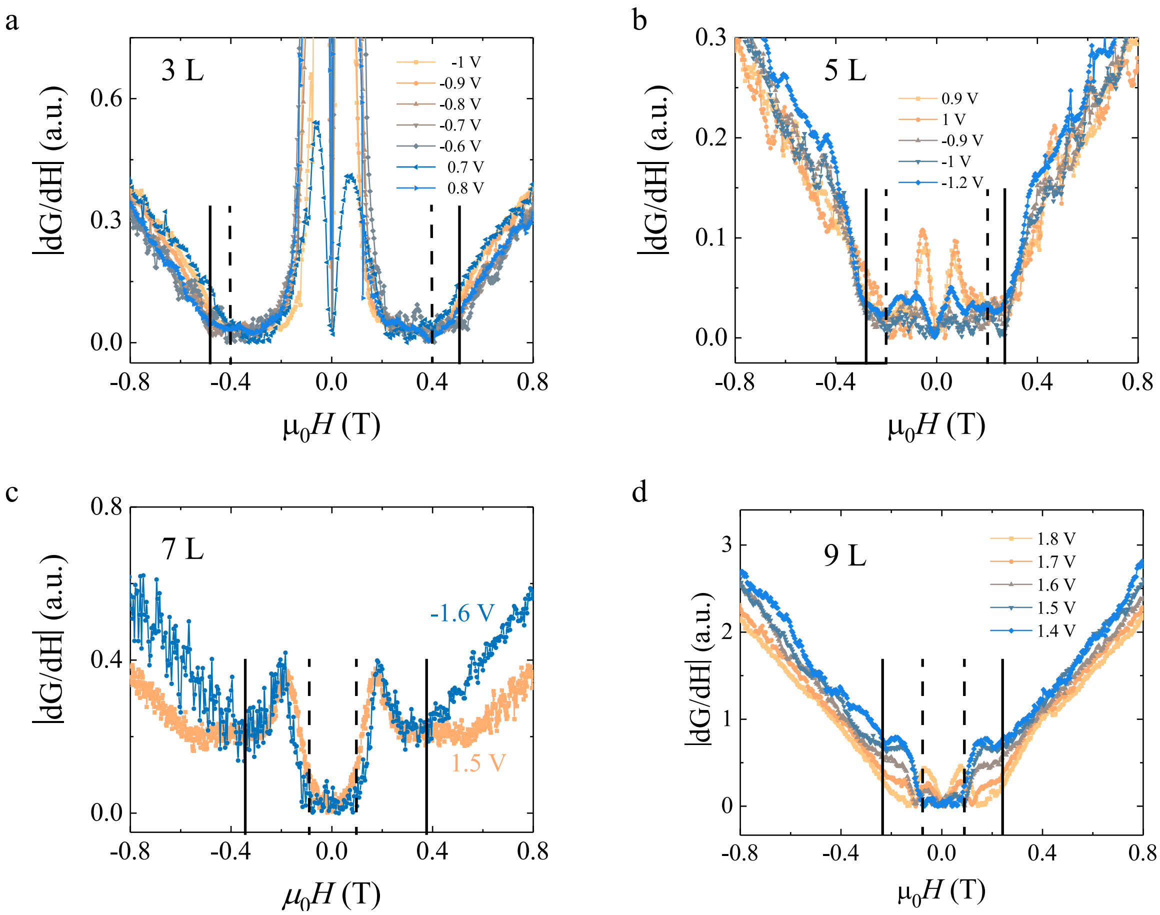


**Supplementary Fig.** 9. **Identification of spin-flop transition field in odd $CrCl_3$ multilayers** (a-d): Magnetic field dependence of $dG/dH$ extracted from measurements performed at different bias (as indicated in the legend of each panel), respectively for $N = 3, 5, 7$, and 9 $CrCl_3$ multilayers. Whereas in even-$N$ multilayers $dG/dH$ only vanishes when the applied field is lowered down to $H = 0$, the data clearly show that in odd-$N$ multilayers $dG/dH$ vanishes (or nearly vanishes) already at finite field. In the ideal situation and at $T = 0$, the largest value of $H$ for which $dG/dH$ vanishes corresponds to the spin-flop field $H_1$. In practice, different aspects of the experiments make the precise determination of $H_1$ more complex. The most significant issue is the feature present at small magnetic field that we discussed in the main text (see, e.g., Fig. 3(d)) and in the supplementary material (Fig. S5). This feature often prevents $dG/dH$ to vanish over a full interval of field around $H = 0$. An additional complication originates from the bias dependence of this feature. In practice, to determine $H_1$ we look both at the largest value of $H$ at which $dG/dH$ vanishes (before starting to increase as $H$ is ramped up towards $H_2$), and at the value of $H$ for which $dG/dH$ has a minimum at low field (in the panels, these values are marked with the vertical continuous and dashed black lines). We take $H_1$ to be the average of these two values; we also take the width of the interval between the two values as experimental indetermination. The points plotted in Fig. 4(c) of the main text –and the corresponding experimental error– have been determined in this way. Despite the fact that for some of the multilayers the experimental indetermination is large, it is clear from the trend in Fig. 4(c) that the overall quality of the data is sufficient to have a meaningful comparison between the measured values of $H_1$ and the theoretical predictions of the antiferromagnetic linear-chain model (see Fig. 4(c)).

[1] McGuire, M. A. *et al.* Magnetic behavior and spin-lattice coupling in cleavable van der Waals layered $CrCl_3$ crystals. *Phys. Rev. Materials* **1**, 014001 (2017).

[2] Narath, A. & Davis, H. L. Spin-wave analysis of the sublattice magnetization behavior of antiferromagnetic and ferromagnetic $CrCl_3$. *Phys. Rev.* **137**, A163–A178 (1965).

[3] MacNeill, D. *et al.* Gigahertz frequency antiferromagnetic resonance and strong magnon-magnon coupling in the layered crystal $CrCl_3$. *arXiv:1902.05669* (2019).

[4] Klein, D. R. *et al.* Giant enhancement of interlayer exchange in an ultrathin 2D magnet. *arXiv:1903.00002* (2019).

[5] Kuhlow, B. Magnetic ordering in $CrCl_3$ at the phase transition. *physica status solidi (a)* **72**, 161–168 (1982).

[6] Wang, H., Eyert, V. & Schwingenschlögl, U. Electronic structure and magnetic ordering of the semiconducting chromium trihalides $CrCl_3$, $CrBr_3$, and $CrI_3$. *Journal of Physics: Condensed Matter* **23**, 116003 (2011).

[7] Zhang, W.-B., Qu, Q., Zhu, P. & Lam, C.-H. Robust intrinsic ferromagnetism and half semiconductivity in stable two-dimensional single-layer chromium trihalides. *J. Mater. Chem. C* **3**, 12457–12468 (2015).

[8] Liu, J., Sun, Q., Kawazoe, Y. & Jena, P. Exfoliating biocompatible ferromagnetic Cr-trihalide monolayers. *Phys. Chem. Chem. Phys.* **18**, 8777–8784 (2016).
